# Supplementary material for: Learning 3D Robotics Perception using Inductive Priors
Source: arXiv:2405.20364 source file (2024-05-30)
Supplement: Supplementary file 1 [file appendix.tex]

\begin{theappendices}

\chapter{Experimental Equipment}
A telescope and a spectrometer were used to analyze the sun. Many other instruments were used.

\chapter{Data Processing}
Data was processed before being added to this document.

\end{theappendices}
